# Supplementary material for: A continuous multiphase model for liquid metal batteries
Source: arXiv:2306.05222 source file (2023-06-08)
Supplement: Supplementary file 1 [file supplementary_information.tex]

\section{Supplementary information}
\subsection{Grid sensitivity and mass conservation}
For the purpose of verifying grid convergence, tests were carried out with mesh sizes of 100, 200, 500, 1000, 2000, and 5000 cells. The dimensions and initial conditions of the system are the same as described in the main text. A sample case imposing a constant voltage in charge mode was prepared and repeated with a constant time-step. The total charge time for each case was recorded and compared for each case as shown in Figure \ref{sensitivity_chargeTime}.

\begin{figure}[h]
    \centering
    \includegraphics[width=0.5\textwidth]{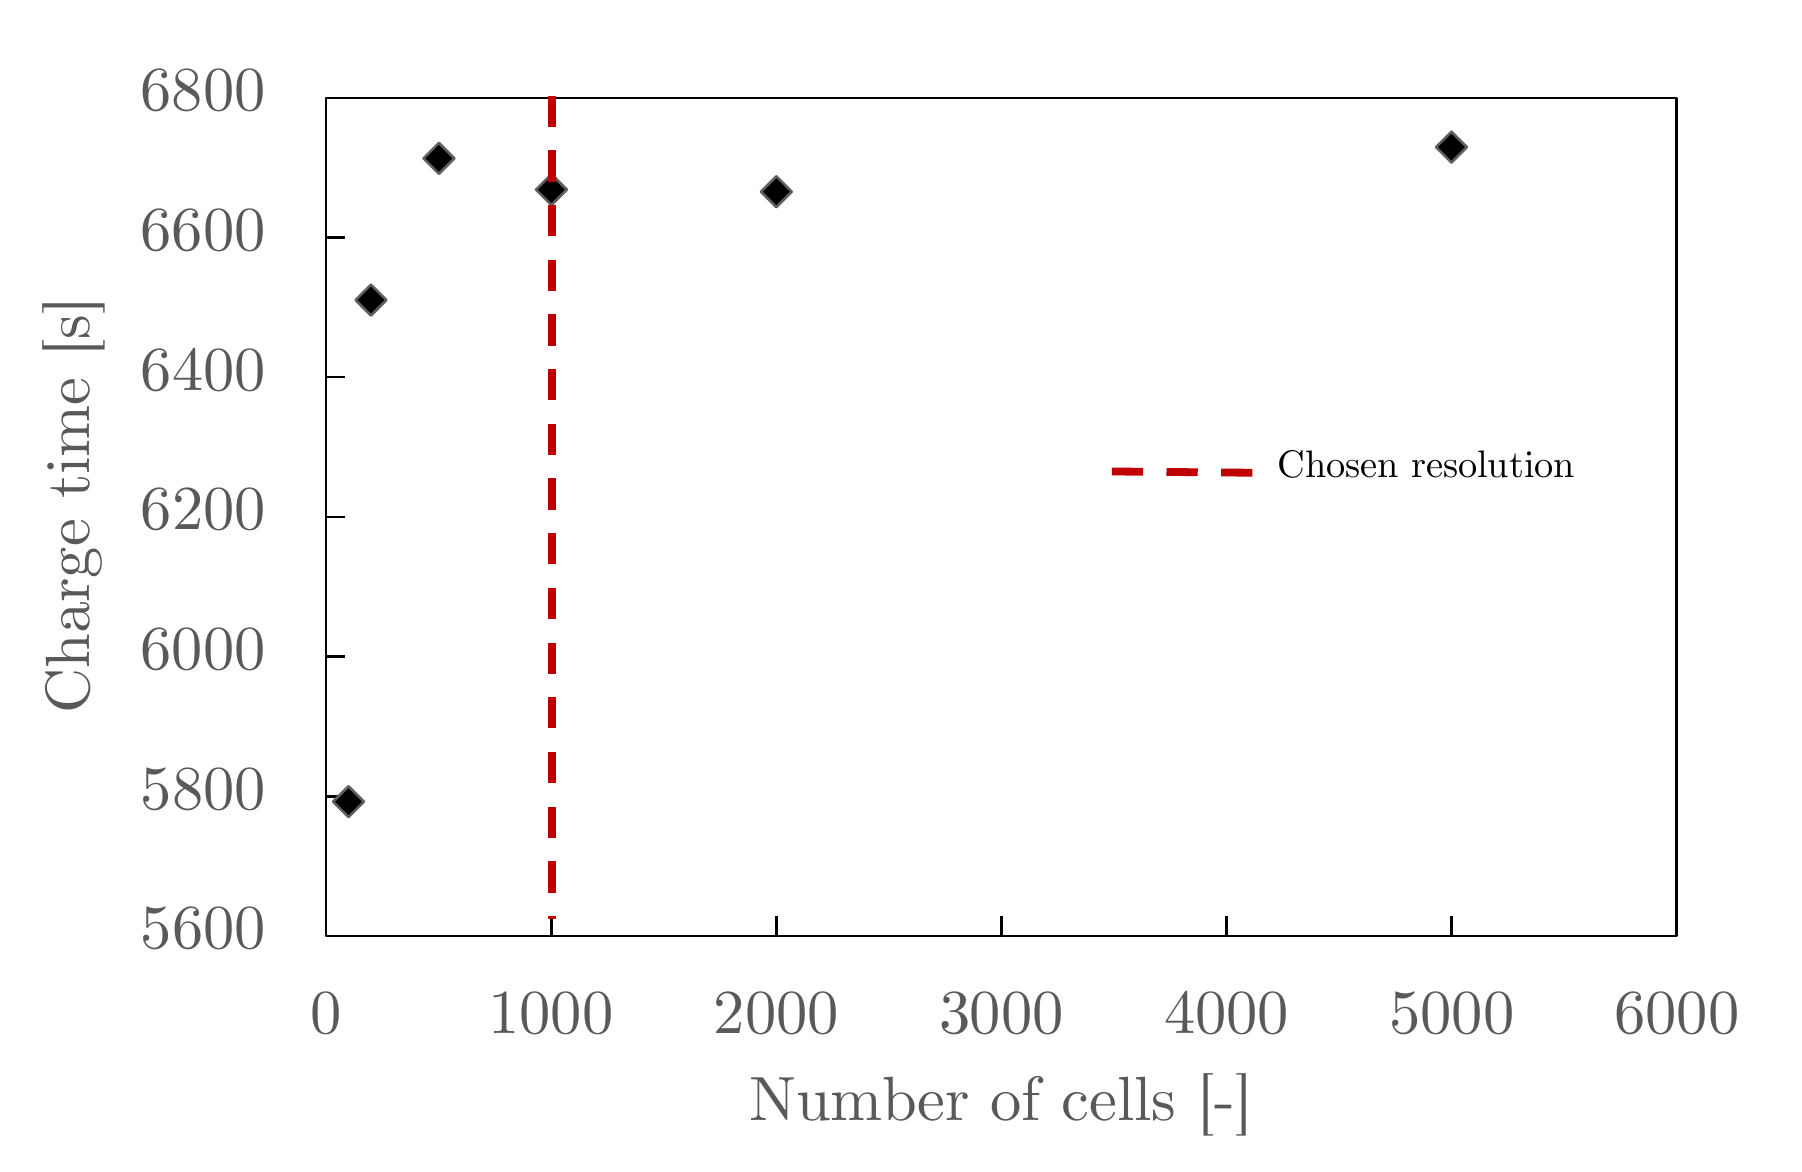}
    \caption{Recorded charge time for different grids.}
    \label{sensitivity_chargeTime}
\end{figure}

No more significant changes are observed past the 500 cells case, with only minor differences when increasing the resolution further.

For additional confirmation, the final average concentration of each of the components ($ \bar{c}_{i,f}$) is shown in Figure \ref{sensitivity_composition}. The average concentration is presented normalized with its corresponding initial conditions ($\bar{c}_{i,0}$). Although there are differences between cases, these are very minor already at the 1000-cell grid size. With these two criteria, it was decided to use 1000 cells for all the calculations presented in the main text. 

\begin{figure}[h]
    \centering
    \includegraphics[width=0.5\textwidth]{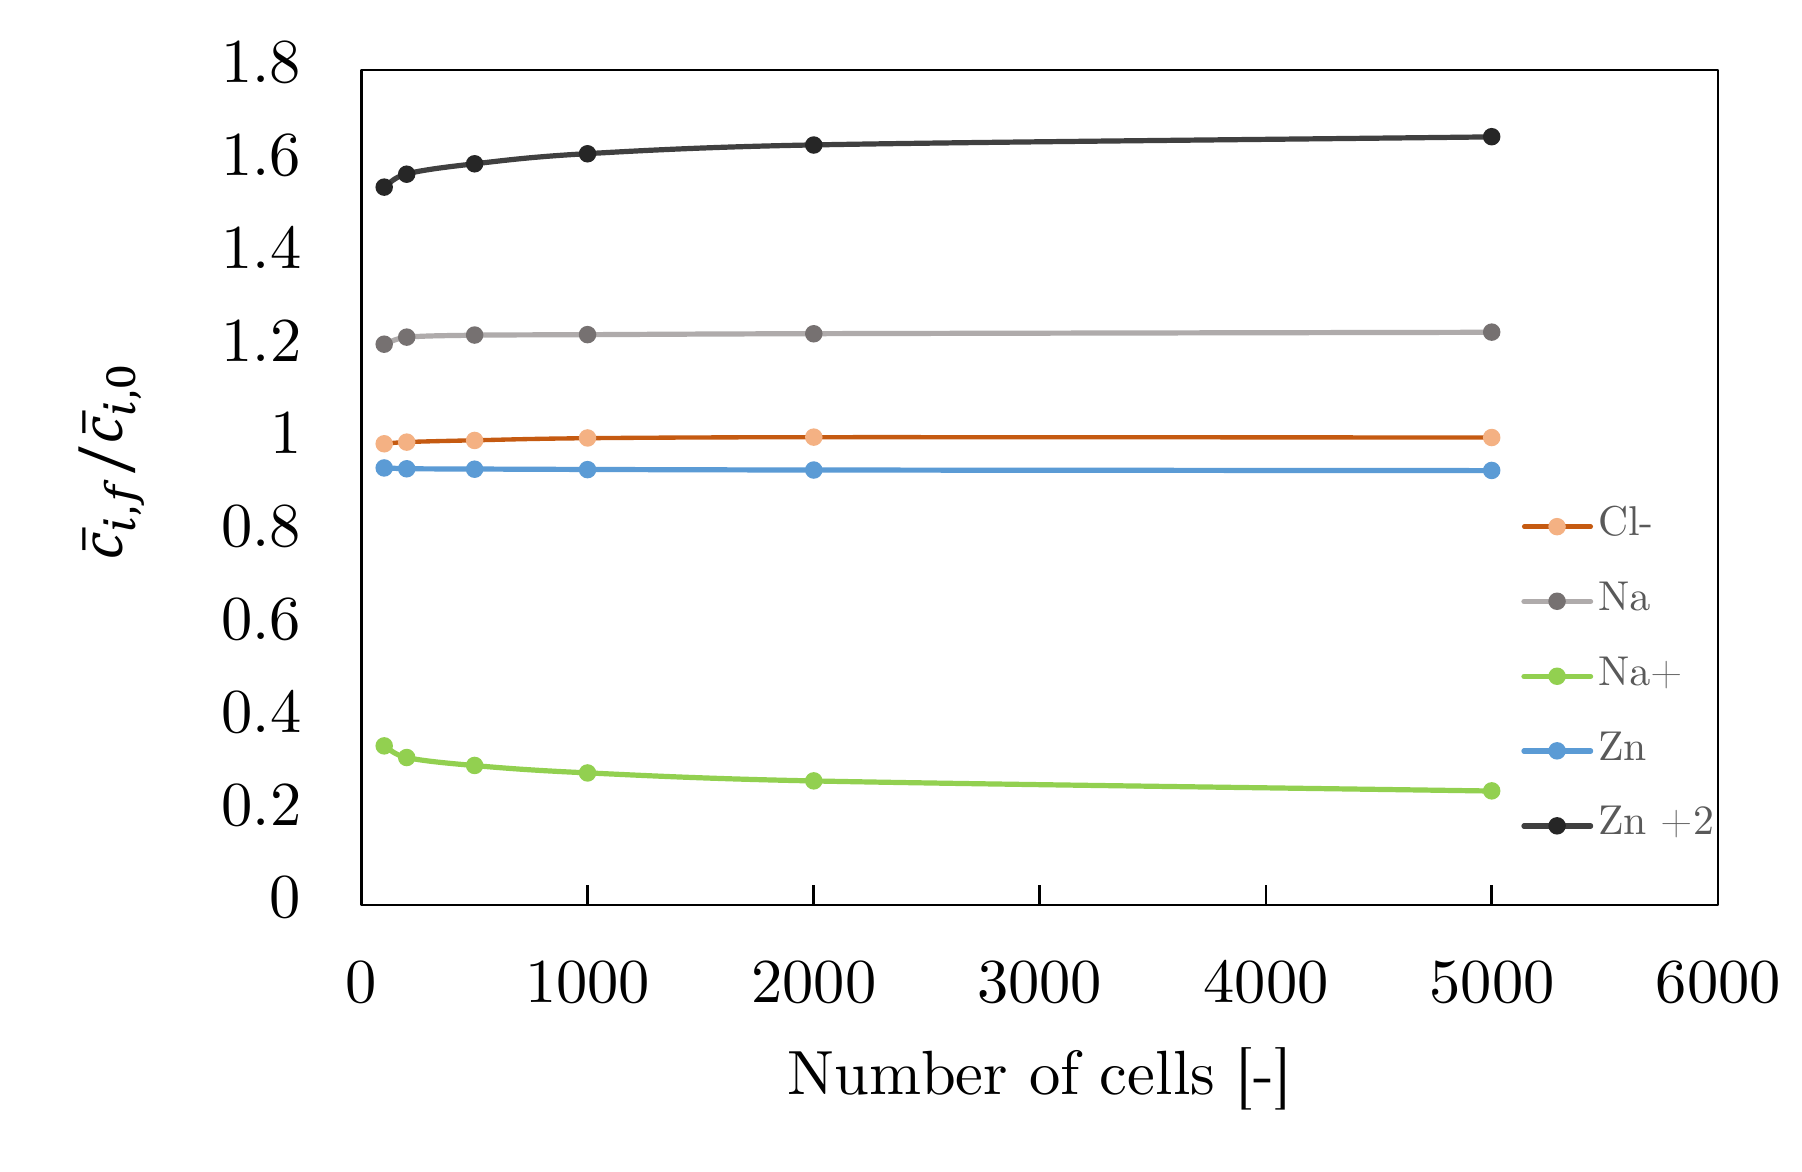}
    \caption{Final average concentration for each grid, relative to the initial concentration.}
    \label{sensitivity_composition}
\end{figure}
